# Supplementary material for: Relativistic motion through a thermal bath as a thermodynamic resource
Source: arXiv:2512.07567 source file (2025-12-20)
Supplement: Supplementary file 1 [file suppliment.pdf]

# — Supplemental Material —
# Relativistic motion through a thermal bath as a thermodynamic resource

Rahul Shastri[1]

[1] *Department of Optics, Palacky University, 17. listopadu 1192/12, 779 00 Olomouc, Czech Republic*

## I. LIMITS OF $\beta^{\rm eff}(\omega;\beta,u)$

Since for systems with single transition frequencies (like TLSs and QHOs), $\beta_{\rm eff}(\omega;\beta,u)$ really can be thought of as effective inverse temperature, let us analyze its behavior in various limits. From the definition we can see that since $N(\omega,\beta,u)\geq 0$,

$$\beta_{\rm eff}(\omega;\beta,u) = \ln\frac{N(\omega,\beta,u)+1}{N(\omega,\beta,u)} \geq 0. \tag{S1}$$

It takes the values $\beta\sqrt{\frac{1-u}{1+u}} \leq \beta_{\rm eff}(\omega;\beta,u) \leq \sqrt{\frac{1+u}{1-u}}$. Depending on the values of $\omega$, $\beta$, and $u$, the effective temperature may be higher, lower, or equal to the bath rest-frame temperature. We now illustrate this by examining a few limiting cases.

*a. Low-velocity limit $u\to 0$.*

$$\beta_{\rm eff}(\omega,\beta,u) \approx \beta\left[1+\frac{u^2}{2}-\frac{u^2}{6}\beta\omega\coth\frac{\beta\omega}{2}\right]. \tag{S2}$$

Here we see that there $\beta_{\rm eff}>\beta$ for $\beta\omega\coth\frac{\beta\omega}{2}<3$ and $\beta_{\rm eff}<\beta$ for $\beta\omega\coth\beta\omega>3$ with the cross over $\beta^*$ satisfying $\beta\omega\coth\beta\omega=3$.

*b. Ultrarelativistic limit $u\to 1$ at fixed $\beta,\omega$.* In this limit using $N\ll 1$ we get,

$$\begin{aligned}\beta_{\rm eff}(\omega,\beta,u) &= -\frac{1}{\omega}\ln\frac{N}{N+1} \approx -\frac{1}{\omega}\ln N\\ &= -\frac{1}{\omega}\ln\left[\frac{\sqrt{1-u^2}}{2u\beta\omega}\ln\frac{1}{\beta\omega\sqrt{\frac{1-u}{1+u}}}\right] \xrightarrow[u\to 1]{} \infty.\end{aligned} \tag{S3}$$

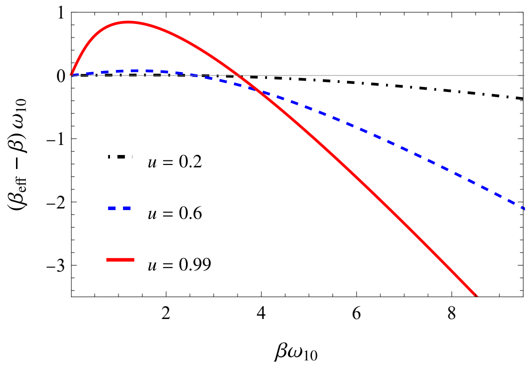


FIG. S1. (Color Online) Effective temperature deviation $\beta_{\rm eff}(\omega_{10},\beta,u)-\beta$ as function of $\beta$ for different values of velocity $u$. Other parameter values are $\omega_{10}=1.0$.

which imply that a detector at ultrarelativistic speed sees the bath colder effectively vacuum like and hence bring the system to ground state.

*c. High-temperature limit $\beta\omega\ll 1$.* In this limit we have,

$$N(\omega,\beta,u) \approx \frac{1}{2\beta\omega}\frac{\sqrt{1-u^2}}{u}\ln\frac{1+u}{1-u}-\frac{1}{2}, \tag{S4}$$

using which we get,

$$\begin{aligned}\beta_{\rm eff}(\omega,\beta,u) &= -\frac{1}{\omega}\ln\frac{N}{N+1} \approx \frac{1}{N}\\ &= \frac{2u\beta}{\sqrt{1-u^2}}\frac{1}{\ln\frac{1+u}{1-u}}.\end{aligned} \tag{S5}$$

which imply that starting form value $\beta$, it increase as we increase $u$. So motion makes system effectively colder.

*d. Low-temperature limit $\beta\omega\gg 1$.* In this limit for moderate speed $\beta\omega\sqrt{\frac{1-u}{1+u}}\gg 1$ we have,

$$N(\omega,\beta,u) \approx \frac{\sqrt{1-u^2}}{2\beta\omega u}e^{-\beta\omega\sqrt{\frac{1-u}{1+u}}}, \tag{S6}$$

which gives,

$$\begin{aligned}\beta_{\rm eff} &= -\frac{1}{\omega}\ln\frac{N}{N+1} \approx -\frac{1}{\omega}\ln N\\ &= \ln\frac{2u\beta}{\sqrt{1-u^2}}+\beta\sqrt{\frac{1-u}{1+u}},\end{aligned} \tag{S7}$$

which imply $\beta_{\rm eff}$ decrease first untill $\beta\omega\sqrt{\frac{1-u}{1+u}}\lesssim 1$ then we have,

$$N(\omega,\beta,u) \approx \frac{\sqrt{1-u^2}}{2\beta\omega\, u}\ln\frac{1}{\beta\omega\sqrt{\frac{1-u}{1+u}}}, \tag{S8}$$

which gives,

$$\begin{aligned}\beta_{\rm eff}(\omega,\beta,u) &= -\frac{1}{\omega}\ln\frac{N}{N+1} \approx -\frac{1}{\omega}\ln N\\ &= -\frac{1}{\omega}\ln\left[\frac{\sqrt{1-u^2}}{2u\beta\omega}\ln\frac{1}{\beta\omega\sqrt{\frac{1-u}{1+u}}}\right] \xrightarrow[u\to 1]{} \infty.\end{aligned} \tag{S9}$$

Hence in low temperature regime, due to motion the system first effectively heats up then cools down as we increase $u$ and eventually cools to zero temperature as we $u\to 1$.

## II. CONNECTION TO SUPER-STATISTICS

Effective occupation number $N(\omega,\beta,u)$ of moving bath can be thought of as convex mixture of Planck distribution with different inverse temperatures as also pointed out in [S1]. More specifically we can write,

$$N(\omega,\beta,u) = \int_{\beta^-}^{\beta^+} d\beta' P(\beta',u) n(\beta',\omega), \tag{S10}$$

where the $P(\beta',u)$ in probability density over interval $[\beta^-,\beta^+]$ with $\beta^\pm = \beta\sqrt{\frac{1\pm u}{1\mp u}}$ and $n(\beta,\omega) = (e^{\beta\omega}-1)^{-1}$ is Planck distribution. As pointed out in [S1] , the form of distribution depends on particular form of coupling. For UD coupling it is a uniform distribution,

$$P(\beta',u) = \frac{\sqrt{1-u^2}}{2u\beta}. \tag{S11}$$

Note that distribution is normalized over range $[\beta^-,\beta^+]$. In the case of bath at rest $u=0$, the distribution is delta function i.e $\lim_{u\to 0}\int d\beta' P(\beta',u) \to \int d\beta' \delta(\beta'-\beta)$ as both limiting points approaches $\beta$ i.e $\beta^\pm \to \beta$. This idea of mixture of bath at different temperature nicely connects to the idea of super-statistics developed by Beck & Cohen [S2].

## III. TWO LEVEL SYSTEM (TLS)

Let us consider the simplest case of TLS with eigenstates $\{|\epsilon_0\rangle, |\epsilon_1\rangle\}$ and energies $\epsilon_0 < \epsilon_1$. The system Hamiltonian is,

$$\hat{H}_\mathrm{S} = \epsilon_0 |\epsilon_0\rangle\langle\epsilon_0| + \epsilon_1 |\epsilon_1\rangle\langle\epsilon_1|. \tag{S12}$$

Define the lowering and raising operators,

$$\hat{S}_{10} = |\epsilon_0\rangle\langle\epsilon_1|, \quad \hat{S}_{01} = |\epsilon_1\rangle\langle\epsilon_0| = \hat{S}_{10}^\dagger, \tag{S13}$$

which satisfies $\left[\hat{H},\hat{S}_{10}\right] = -\omega_{10}\hat{S}_{10}$, where $\omega_{10} = (\epsilon_1 - \epsilon_0) > 0$ is positive Bohr frequency. The interaction operator,

$$\hat{A}^\mathrm{I}(\tau) = \lambda(\hat{S}_{10}e^{-i\omega_{10}\tau} + \hat{S}_{10}^\dagger e^{i\omega_{10}\tau}). \tag{S14}$$

The steady-state of the system can be obtained by choosing $F_0 = 0$ and $F_1 = -\ln\frac{k_{0\to1}}{k_{1\to0}} = \beta(\omega_{10})\omega_{10}$ as,

$$\hat{\rho}^\mathrm{ss} = p_0^\mathrm{ss}|\epsilon_0\rangle\langle\epsilon_0| + p_1^\mathrm{ss}|\epsilon_1\rangle\langle\epsilon_1|, \tag{S15}$$

where,

$$p_0^\mathrm{ss} = \frac{1}{1+e^{-\beta_\mathrm{eff}(\omega_{10},\beta,u)\omega_{10}}}, \quad p_1^\mathrm{ss} = \frac{e^{-\beta_\mathrm{eff}(\omega_{10},\beta,u)\omega_{10}}}{1+e^{-\beta_\mathrm{eff}(\omega_{10},\beta,u)\omega_{10}}}. \tag{S16}$$

Let us now ask how the effective inverse temperature $\beta_\mathrm{eff}(\omega_{10};\beta,u)$ behaves as compared to the bath temperature $\beta$ as function of velocity $u$.

Fig. (S1) shows difference $\beta_\mathrm{eff}(\omega_{10};\beta,u)-\beta$ as function of $\beta$ for different values of $u$. We can see the cross over form $\beta_\mathrm{eff} > \beta$ to $\beta_\mathrm{eff} < \beta$ as we increase $\beta$ for fixed $u$. This shows that the effective temperature can be lower or higher than the bath rest temperature. For fixed $\beta$, in the limit of $u \to 1$, we always get $\beta_\mathrm{eff} \to \infty$ implying that at sufficiently high relativistic velocity the system always cools down to ground state. Note than since $\beta_\mathrm{eff} \geq 0$ for any $u$, the state can not have population inversion in this case.

## IV. THREE-LEVEL SYSTEM

Let us consider a three-level system with eigenstates $\{|\epsilon_0\rangle, |\epsilon_1\rangle, |\epsilon_2\rangle\}$ with corresponding energies $\epsilon_0 < \epsilon_1 < \epsilon_2$. The system Hamiltonian is,

$$\hat{H}_\mathrm{S} = \epsilon_0|\epsilon_0\rangle\langle\epsilon_0| + \epsilon_1|\epsilon_1\rangle\langle\epsilon_1| + \epsilon_2|\epsilon_2\rangle\langle\epsilon_2|. \tag{S17}$$

Define the lowering and raising operators,

$$\hat{S}_{10} = |\epsilon_1\rangle\langle\epsilon_0|, \quad \hat{S}_{21} = |\epsilon_2\rangle\langle\epsilon_1|, \quad \hat{S}_{20} = |\epsilon_2\rangle\langle\epsilon_0|, \tag{S18}$$

such that $[H_S, S_{ij}] = -\omega_{ij}S_{ij}$ with Bohr frequencies $\omega_{ij} = \epsilon_i - \epsilon_j > 0$ and $S_{ji} = S_{ij}^\dagger$. Consider interaction operator of the form,

$$\hat{A}^\mathrm{I}(\tau) = \sum_{(ij)\in\{10,21,20\}} \lambda_{ij}(\hat{S}_{ij}e^{-i\omega_{ij}\tau} + \hat{S}_{ij}^\dagger e^{i\omega_{ij}\tau}). \tag{S19}$$

Note that we assume non-degenerate and well separated Bohr frequencies $\omega_{ij}$ such that the secular approximation is valid. Populations obey a classical master equation

$$\mathbf{p}(t) = [p_0(\tau), p_1(\tau), p_2(\tau)]^\mathrm{T}, \quad \dot{\mathbf{p}}(\tau) = W\,\mathbf{p}(\tau), \tag{S20}$$

where

$$W = \begin{bmatrix} -(k_{0\to1}+k_{0\to2}) & k_{1\to0} & k_{2\to0} \\ k_{0\to1} & -(k_{1\to2}+k_{1\to0}) & k_{2\to1} \\ k_{0\to2} & k_{1\to2} & -(k_{2\to0}+k_{2\to1}) \end{bmatrix}. \tag{S21}$$

The rate equation in terms of probability current is,

$$\dot{p}_0(\tau) = -J_{0\to1} + J_{2\to0} \tag{S22}$$
$$\dot{p}_1(\tau) = -J_{1\to2} + J_{0\to1} \tag{S23}$$
$$\dot{p}_2(\tau) = -J_{2\to0} + J_{1\to2}. \tag{S24}$$

### A. $\Lambda$ configuration with one transition forbidden

In the interaction we set $\lambda_{01} = 0$, so only $2 \leftrightarrow 0$ and $2 \leftrightarrow 1$ transitions are allowed and $1 \leftrightarrow 0$ is forbidden then for steady state each current vanishes,

$$J_{2\to0}^\mathrm{ss} = 0 \;\Rightarrow\; \frac{p_2^\mathrm{ss}}{p_0^\mathrm{ss}} = \frac{k_{0\to2}}{k_{2\to0}} = e^{-\beta_\mathrm{eff}(\omega_{20})\omega_{20}}, \tag{S25}$$

$$J_{1\to2}^\mathrm{ss} = 0 \;\Rightarrow\; \frac{p_2^\mathrm{ss}}{p_1^\mathrm{ss}} = e^{-\beta_\mathrm{eff}(\omega_{21})\omega_{21}}. \tag{S26}$$

And the steady-state is,

$$\hat{\rho}^{\rm ss} = p_0^{\rm ss} \left|\epsilon_0\right\rangle \left\langle\epsilon_0\right| + p_1^{\rm ss} \left|\epsilon_1\right\rangle \left\langle\epsilon_1\right| + p_2^{\rm ss} \left|\epsilon_2\right\rangle \left\langle\epsilon_2\right|, \quad \text{(S27)}$$

where,

$$p_0^{\rm ss} = \frac{1}{A_0}, \quad \text{(S28)}$$

$$p_1^{\rm ss} = \frac{e^{\beta_{\rm eff}(\omega_{21})\omega_{21} - \beta_{\rm eff}(\omega_{20})\omega_{20}}}{A_0}, \quad \text{(S29)}$$

$$p_2^{\rm ss} = \frac{e^{-\beta_{\rm eff}(\omega_{20})\omega_{20}}}{A_0}, \quad \text{(S30)}$$

with normalisation,

$$A_0 = 1 + e^{\beta_{\rm eff}(\omega_{21})\omega_{21} - \beta_{\rm eff}(\omega_{20})\omega_{20}} + e^{-\beta_{\rm eff}(\omega_{20})\omega_{20}}. \quad \text{(S31)}$$

Note that the above steady state can be transformed in to Gibbs form (**??**) only if $\beta_{\rm eff}(\omega_{20}) = \beta_{\rm eff}(\omega_{21})$ (which holds for $u = 0$). Also similar to TLS, in the ultrarelativistic limit $u \to 1$ (fixed $\beta, \omega$), $N(\omega) \to 0$ and $\beta_{\rm eff}(\omega) \to \infty$, so the excited-state populations are exponentially suppressed and the system cools down to ground state.

### B. Δ configuration with all three transitions

Allowing also the $1 \leftrightarrow 0$ transition in above case closes the cycle $0 \to 2 \to 1 \to 0$ and we find that condition (**??**) no longer satisfied. This implies that the steady-state is NESS with persistent current. We define the cycle affinity as,

$$\begin{aligned}\mathcal{A} &= \ln \frac{k_{2\to0}\, k_{1\to2}\, k_{0\to1}}{k_{0\to2}\, k_{2\to1}\, k_{1\to0}} \\ &= \beta_{\rm eff}(\omega_{20};\beta,u)\omega_{20} - \beta_{\rm eff}(\omega_{21};\beta,u)\omega_{21} \\ &\quad - \beta_{\rm eff}(\omega_{10};\beta,u)\omega_{10}. \end{aligned} \quad \text{(S32)}$$

For $u = 0$ one has $\beta_{\rm eff}(\omega) \equiv \beta$ and $\mathcal{A} = 0$. The steady states $\mathbf{p}^{\rm ss}$ can be obtained by solving $W\mathbf{p}^{\rm ss} = 0$. Note that for this system, the NESS carries a single circulating current,

$$\mathcal{J} \equiv J^{\rm ss}_{0\to1} = J^{\rm ss}_{1\to2} = J^{\rm ss}_{2\to0}. \quad \text{(S33)}$$

Let us now calculate the steady-state current $\mathcal{J}$ and diffusion constant $D$ for this setup. We count the net transition from $2 \to 0$ and call this complete cycle as one tick. If stochastic variable $n(\tau)$ keeps count of the transitions such that for $2 \to 0$ the variable increase by $+1$ and for $0 \to 2$ decrease by $-1$. The joint probability $p_i(n,\tau)$ of in state $i$ with count $n$ at time $\tau$ evolve as,

$$\begin{aligned}\dot{p}_0(n) &= k_{1\to0}p_1(n) + k_{2\to0}p_2(n-1) - (k_{0\to1} + k_{0\to2})p_0(n)\\ \dot{p}_1(n) &= k_{0\to1}p_0(n) + k_{2\to1}p_2(n) - (k_{1\to0} + k_{1\to2})p_1(n)\\ \dot{p}_2(n) &= k_{0\to2}p_0(n+1) + k_{1\to2}p_1(n) - (k_{2\to0} + k_{2\to1})p_2(n).\end{aligned} \quad \text{(S34)}$$

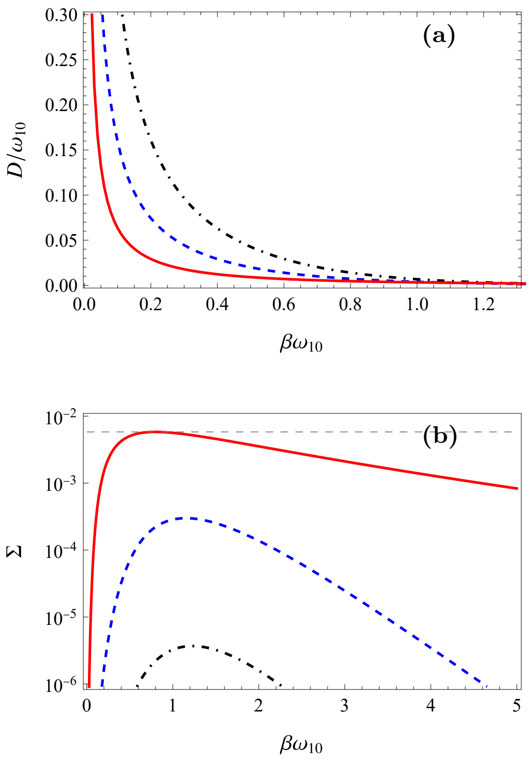


FIG. S2. (Color Online) Diffusion constant $D$ (a) and entropy production $\Sigma$ (b) as function of inverse temperature $\beta$ for different values of velocity $u$. Other parameter values are $\omega_{10} = 1.0$, $\omega_{21} = 3.1\omega$.

Let us define generating function,

$$G_i(\xi,\tau) = \sum_{n=-\infty}^{\infty} e^{i\xi n} p_i(n,\tau) \quad \text{(S35)}$$

$$F(\xi,\tau) = \sum_i G_i(\xi,\tau) = \sum_{n=-\infty}^{\infty} e^{i\xi n} p(n,\tau). \quad \text{(S36)}$$

From this we can obtain all the cumulative moments as,

$$\langle n^k \rangle_{\rm c}(\tau) = \frac{\partial^k \ln F(\xi,\tau)}{(\partial i\xi)^k}|_{\xi=0}. \quad \text{(S37)}$$

The generating function vector $\mathbf{G}(\xi,\tau) = [G_0(\xi,\tau), G_1(\xi,\tau), G_2(\xi,\tau)]^{\rm T}$ satisfy,

$$\dot{\mathbf{G}}(\xi,\tau) = W(\xi)\mathbf{G}(\xi,\tau), \quad \text{(S38)}$$

where $W(\xi)$ is the tilted rate matrix,

$$W(\xi) = \begin{bmatrix} -(k_{0\to1} + k_{0\to2}) & k_{1\to0} & k_{2\to0}e^{i\xi} \\ k_{0\to1} & -(k_{1\to2} + k_{1\to0}) & k_{2\to1} \\ k_{0\to2}e^{-i\xi} & k_{1\to2} & -(k_{2\to0} + k_{2\to1}) \end{bmatrix}. \quad \text{(S39)}$$

Here we have used the relations,

$$\sum_{n=-\infty}^{\infty} e^{i\xi n} p_2(n-1,\tau) = e^{i\xi} G_2(\xi,\tau) \tag{S40}$$

$$\sum_{n=-\infty}^{\infty} e^{i\xi n} p_0(n+1,\tau) = e^{-i\xi} G_0(\xi,\tau). \tag{S41}$$

The solution of the master equation for generating function will be,

$$\mathbf{G}(\xi,\tau) = e^{W(\xi)}\mathbf{G}(\xi,0). \tag{S42}$$

Which implies,

$$F(\xi,\tau) = 1^{\mathrm{T}} e^{W(\xi)}\mathbf{G}(\xi,0), \tag{S43}$$

where $1^{\mathrm{T}} = [1,1,1]$. In long time limit we have,

$$\lim_{\tau\to\infty} F(\xi,\tau) \approx e^{q(\xi)\tau}, \tag{S44}$$

where $q(\xi)$ is the largest eigenvalue of $W(\xi)$. From which we get the first two cumulative moments as,

$$\lim_{\tau\to\infty} \frac{\langle n\rangle(\tau)}{\tau} = \frac{\partial q(\xi)}{\partial i\xi}|_{\xi=0} = \mathcal{J} \tag{S45}$$

$$\lim_{\tau\to\infty} \frac{\mathrm{Var}[n](\tau)}{\tau} = \frac{\partial^2 q(\xi)}{(\partial i\xi)^2}|_{\xi=0} = 2D, \tag{S46}$$

where $\mathrm{Var}[n] = \langle n^2\rangle - \langle n\rangle^2$, $\mathcal{J}$ is current and $D$ is diffusion constant. Note that finding eigenvalues of tilted matrix $W(\xi)$ is not always easy. But we don't need to find the eigenvalue for just calculating first few moments. Let us take the eigenvalue equation for right eigenvector $\mathbf{r}(\xi)$,

$$W(\xi)\mathbf{r}(\xi) = q(\xi)\mathbf{r}(\xi). \tag{S47}$$

Here $\xi = 0$ gives the zeroth order equation,

$$W(0)\mathbf{r}(0) = q(0)\mathbf{r}(0). \tag{S48}$$

Since $W(0) = W$ we have $\mathbf{1}^{\mathrm{T}}W = 0$, $\mathbf{r}(0) = \mathbf{p}^{\mathrm{ss}}$ and $q(0) = 0$. We fix left and right eigenvector such that $\mathbf{l}(\xi)^{\mathrm{T}}\mathbf{r}(\xi) = 1$. Which implies $\mathbf{l}(0)^T = \mathbf{1}^{\mathrm{T}}$. Now differentiating eigenvalues equation at $\xi = 0$ gives,

$$W'(0)\mathbf{p}^{\mathrm{ss}} + W\mathbf{r}'(0) = q'(0)\mathbf{p}^{\mathrm{ss}}. \tag{S49}$$

Multiplying from left by $\mathbf{1}^{\mathrm{T}}$ and using $\mathbf{1}^{\mathrm{T}}W = 0$ and $\mathbf{1}^{\mathrm{T}}\mathbf{p}^{\mathrm{ss}} = 1$ gives,

$$q'(0) = \mathbf{1}^{\mathrm{T}}W'(0)\mathbf{p}^{\mathrm{ss}}. \tag{S50}$$

Similarly differentiating eigenvalue equation twice at $\xi = 0$ gives,

$$W''(0)\mathbf{p}^{\mathrm{ss}} + 2W'(0)\mathbf{r}'(0) = q''(0)\mathbf{p}^{\mathrm{ss}} + 2q'(0)\mathbf{r}'(0). \tag{S51}$$

From which after multiplying $\mathbf{1}^{\mathrm{T}}$ from left gives,

$$q''(0) = \mathbf{1}^{\mathrm{T}}W''(0)\mathbf{p}^{\mathrm{ss}} + 2\mathbf{1}^{\mathrm{T}}W'(0)\mathbf{r}'(0). \tag{S52}$$

where $\mathbf{r}'(0)$ can be solved using,

$$W\mathbf{r}'(0) = (\mathcal{J}I - W'(0))\mathbf{p}^{\mathrm{ss}}, \tag{S53}$$

together with $\mathbf{1}^{\mathrm{T}}\mathbf{r}'(0) = 0$. Using this recipe we calculate $\mathcal{J}$ and $D$.
Coming back to the equation, in the long time limit we have,

$$\langle n\rangle_\tau \approx \mathcal{J}\tau \tag{S54}$$

$$\mathrm{Var}(n)_\tau \approx 2D\tau. \tag{S55}$$

For performance of the stochastic clock we look at two quantities,

$$\mathcal{J} = \frac{\langle n\rangle_\tau}{\tau} \tag{S56}$$

$$\delta^2 = \frac{2D}{\mathcal{J}^2} \tag{S57}$$

where $\mathcal{J}$ gives number of cycles per unit time and $\delta^2$ characterize relative uncertainty. In time interval $\tau$, we expect to read $\mathcal{J}\tau$ number of cycles on average with relative uncertainly $\delta = \frac{\sqrt{2D}}{\mathcal{J}}\frac{1}{\sqrt{\tau}}$.

Fig (S2)(a) shows that diffusion constant $D$ as function of inverse temperature $\beta$ for different values of velocity $u$. We can see that $D$ decreases monotonically with $\beta$. The entropy production $\Sigma = \mathcal{J}\mathcal{A}$ is shown in Fig. S2(b). We see that $\Sigma$ remains finite whenever the system is driven out of equilibrium.

[S1] N. Papadatos and C. Anastopoulos, Phys. Rev. D **102**, 085005 (2020).

[S2] C. Beck, in *Anomalous Distributions, Nonlinear Dynamics, and Nonextensivity* (World Scientific, 2005).
